# Supplementary material for: No-Regret Algorithms for Time-Varying Bayesian Optimization
Source: arXiv:2102.06296 source file (2021-04-30)
Supplement: Supplementary file 1 [file appendix.tex]

\subsection{Important Facts}
Under Assumption~\ref{ass:regularity}, we have that the states and controls are bounded, which directly follows from Proposition 8 in~\cite{wang2020episodic}.
\begin{lemma}
\label{lem:fact_xz}
    Under Assumption~\ref{ass:regularity}, our algorithm satisfies
    \begin{align*}
        \norm{x_{k,h}}_2 \le 1, \norm{u_{k,h}}_2 \le \gamma, \norm{z_{k,h}}_2 \le (1+\gamma)
    \end{align*}
for all $k\ge 1$ and $h \in[H]$.
\end{lemma}

We also have an upper bound on the matrices $P_h(\Theta)$, which follows from Proposition 6 in~\cite{wang2020episodic}.
\begin{lemma}
\label{lem:fact_P}
    Under Assumption~\ref{ass:regularity}, there exists a constant $D$ such that for all $\Theta \in \mathcal{C}_k(\delta) \cap \mathcal{S}$, 
    \begin{align*}
        \norm{P_{k,h}(\Theta)}_2 \le D
    \end{align*}
    holds for all $k\ge 1$ and $h\in [H]$.
\end{lemma} 

\begin{lemma}[Operator norm of symmetric Gaussian random matrices]
\label{lem:norm_sym_gaussian}
    Let $A$ be an $n \times n$ random symmetric matrix whose entries $A_{ij}$ on and above the diagonal are $i.i.d$ Gaussian random variables $\mathcal{N}(0,\sigma^2)$. Then, for any $t>0$, we have \begin{align*}
        \norm{A} \le 4\sigma\sqrt{n} + 2t,
    \end{align*}
    with probability at least $1-2\exp(-\frac{t^2}{2\sigma^2})$.
\end{lemma} 

 \begin{lemma}[Concentration of chi-square; Corollary to Lemma 1 of~\cite{laurent2000adaptive}]
 \label{lem:chi-square}
    Let $U$ be a $\chi^2$ statistic with $D$ degrees of freedom. Then, for any positive $x$,
    \begin{align*}
        \mathbb{P}\left\{ U \ge D + 2\sqrt{Dx} + 2x\right\} \le \exp(-x).
    \end{align*}
 \end{lemma}

\subsection{Proof of Theorem~\ref{thm:CI}}
% The proof of Theorem~\ref{thm:CI} builds on the following improved concentration bound, which is of independent interest.
% \xingyu{Maybe, we can even put this lemma in the main section if possible.}
% \begin{lemma}
% \label{lem:improved_bound}
%     Let $\lbrace \mathcal{F}_t \rbrace_{t=0}^{\infty}$ be a filtration generated by the random variables $\lbrace s_{t+1},a_{t+1} \rbrace_{t=0}^{\infty}$. Let
%          $\lbrace \eta_t \rbrace_{t \geq 1}$ be a vector-valued martingale difference process adapted to the filtration $\lbrace\mathcal{F}_t\rbrace_{t \geq 0}$. Further, let $\eta_t$ be a be sub-Gaussian random vector in $\Real^n$ with parameter $R$, i.e., it satisfies, for some $R >0$, and any $t\ge 1$, any $\alpha \in \Real^n$:
%         \begin{align}
%         \label{eqn:noise}
%             \mathbb{E}\left[\exp\left( \alpha^T\eta_t\right) | \cF_{t-1}\right] \leq \exp\left(\frac{R^2\norm{\alpha}^2}{2}\right) \quad
%             \text{a.s.}
%         \end{align}
%         Let $V_t = \sum_{i=1}^{t}\phi(s_i,a_i)\phi(s_i,a_i)^T$, $\overline{V}_t = V_t+\lambda I$ and $S_t = \sum_{i=1}^{t}\phi(s_i,a_i)\eta_i^T$. Then, for any $0 < \delta \leq 1$, with probability at least $1-\delta$, uniformly over all $t \geq 1$, it holds that
%         \begin{align}
%           \norm{\overline{V}_t^{-1/2}S_t}_F \leq R \sqrt{2\ln \left(\frac{1}{\delta}\right)+n\ln \frac{\det(\overline{V}_t)}{\det(\lambda I_m)}}.
%           \label{eqn:self-normalized-inequality}
%         \end{align}
% \end{lemma}

\begin{proof}
For any $k \ge 1$, we have
    \begin{align*}
       &\Theta_*- {\Theta}_k\\ 
       = &\Theta_* - {V}_k^{-1}{U}_k\\
       = &\Theta_* - {V}_k^{-1}\left(Z_k^TZ_k\Theta_* + Z_k^TW_k + L_k\right)\\
       = &\Theta_* - {V}_k^{-1}\left( {V}_k\Theta_* - H_k\Theta_* + Z_k^TW_k + L_k \right)\\
       = & \hat{V}_k^{-1}\left(H_k\Theta_* - Z_k^TW_k -L_k\right).
    \end{align*}
Hence, we have 
\begin{align*}
     &\norm{{\Theta}_k - \Theta_*}_{{V}_k}\\
     = &\norm{H_k\Theta_* - Z_k^TW_k -L_k}_{{V}_k^{-1}}\\
     \lep{a}& \norm{Z_k^TW}_{{V}_k^{-1}} + \norm{H_k\Theta_*}_{{V}_k^{-1}} + \norm{L_k}_{{V}_k^{-1}}\\
     \lep{b}& \norm{Z_k^TW_k}_{{V}_k^{-1}} + \norm{H_k\Theta_*}_{H_k^{-1}}+\norm{L_k}_{H_k^{-1}}\\
     \lep{c}& \norm{Z_k^TW_k}_{(G_k + \lambda_{min}I)^{-1}} + \norm{H_k^{\frac{1}{2}}\Theta_*}_F + \norm{L_k}_{H_k^{-1}}\\
     \lep{d}& \underbrace{\norm{Z_k^TW_k}_{(G_k + \lambda_{min}I)^{-1}}}_{\mathcal{T}_1} + \underbrace{\norm{H_k^{\frac{1}{2}}}_2+ \norm{L_k}_{H_k^{-1}}}_{\mathcal{T}_2},
\end{align*}
where (a) follows from triangle inequality; (b) holds by ${V}_k \succeq H_k$; (c) is true since ${V}_k \succeq (G_k + \lambda_{min}I)$ under Assumption~\ref{ass:regularizer}; (d) follows from the fact for any two matrices $A$ and $B$, $\norm{AB}_F \le \norm{A}_2 \norm{B}_F$, and the assumption $\norm{\Theta_*}_F \le 1$ in Assumption~\ref{ass:regularity}.

Now, we are left to bound $\mathcal{T}_1$ and $\mathcal{T}_2$, respectively. First, under Assumption~\ref{ass:regularizer}, by a union bound,  we have w.p. at least $1-\delta/2$,
\begin{align*}
    \mathcal{T}_2 \le \sqrt{\lambda_{max}} + \nu.
\end{align*}
For $\mathcal{T}_1$, we can apply Lemma~\ref{lem:improved_bound} since noise $w_{k,h}$ is a sub-Gaussian vector with parameter $C_w$ under the assumption (b) in Assumption~\ref{ass:regularity}. Thus, we have w.p. at least $1-\delta/2$, 
\begin{align*}
          \mathcal{T}_1 \le C_w \sqrt{2\ln \left(\frac{2}{\delta}\right)+n\ln \frac{\det({G}_k + \lambda_{min}I)}{\det(\lambda_{min} I)}}.
\end{align*}
Finally, putting the bounds on $\mathcal{T}_1$ and $\mathcal{T}_2$ together, yields the required result.
\end{proof}

\subsection{Proof of Theorem~\ref{thm:regret}}
\begin{proof}
We choose an error probability $\delta > 0$. Given this, we define the following `good' event, i.e., the confidence set holds.
\begin{align*}
    \mathcal{E}_K(\delta) := \{\Theta_* \in \mathcal{C}_k(\delta) \cap \mathcal{S}, \forall k = 1,2\ldots,K \},
\end{align*}
in which $\mathcal{C}_k(\delta)$ is given by~\eqref{eq:Confidence_set}. As a direct result of Theorem~\ref{thm:CI} and (a) in Assumption~\ref{ass:regularity}, we know with probability at least $1-\delta$, the event $\mathcal{E}_K(\delta)$ is true. 

In the following, we will bound the regret under event $\mathcal{E}_K(\delta)$. First, we can decompose the regret as in the following lemma.
\begin{lemma}
\label{lem:regret_decomp}
    Let $\widetilde{P}_{k,h} := P_h(\widetilde{\Theta}_k)$ given by~\eqref{eq:P-matrix} and $\mathcal{F}_{k,h}$ is  is all randomness before time $(k,h)$. Under event $\mathcal{E}_{K}(\delta)$, we have
    \begin{align*}
        \mathcal{R}(K) \le \sum_{k=1}^K\sum_{h=1}^{H}(\Delta_{k,h} + \Delta_{k,h}^{\prime} + \Delta_{k,h}^{\prime\prime}), 
    \end{align*}
    where 
    \begin{align*}
        &\Delta_{k,h} :=\mathbb{E}\left[J_{h+1}^{\pi_k}(\Theta_*,x_{k,h+1}) \mid \mathcal{F}_{k,h}\right] - J_{h+1}^{\pi_k}(\Theta_*,x_{k,h+1}),\\
        &\Delta_{k,h}^{\prime}:= \norm{x_{k,h+1}}_{\widetilde{P}_{k,h+1}} - \mathbb{E}\left[\norm{x_{k,h+1}}_{\widetilde{P}_{k,h+1}} \mid \mathcal{F}_{k,h}\right],\\
        &\Delta_{k,h}^{\prime\prime} := \norm{\Theta_*^\top z_{k,h}}_{\tp_{k,h+1}} - \norm{\widetilde{\Theta}_k^\top z_{k,h}}_{\tp_{k,h+1}}.
    \end{align*}
\end{lemma}

Now, we will turn to bound each of the three terms above.
For the first two terms, we can bound them by using the following lemma.
\begin{lemma}
\label{lem:two_Sum}
    Under Assumption~\ref{ass:regularity} and the event $\mathcal{E}_K(\delta)$, with probability at least $1-2\delta$, we have both
    \begin{align*}
        \left| \sum_{k=1}^K \sum_{h=1}^{H} \Delta_{k,h} \right| \le O\left(\sqrt{KH^3\ln\frac{2}{\delta}}\right)
    \end{align*}
    and
    \begin{align*}
        \left| \sum_{k=1}^K \sum_{h=1}^{H} \Delta'_{k,h} \right| \le O\left(\sqrt{KH\ln\frac{2}{\delta}}\right)
    \end{align*}
\end{lemma}

For the third term, we can bound it as follows.
\begin{lemma}
\label{lem:thrid_Sum}
    Under Assumption~\ref{ass:regularity} and the event $\mathcal{E}_K(\delta)$, we have 
    \begin{align*}
        &\sum_{k=1}^K\sum_{h=1}^{H}\Delta''_{k,h}\\
        = &O\left(H\sqrt{K}\beta_k(\delta)\left( \ln\frac{\det(G_k+\lambda_{min} I)}{\det( \lambda_{min}I )}\right)^{1/2}\right).
    \end{align*}
\end{lemma}

Finally, we are ready to put everything together. 
We first note that by the boundness result in Lemma~\ref{lem:fact_xz}
\begin{align*}
    \ln\det(G_k + \lambda_{min}I) \le (n+d)\ln\left(\lambda_{min} + \frac{HK(1+\gamma)^2}{n+d}\right).
\end{align*}
Based on this and $\hat{\gamma}:=(1+\gamma)^2$, we have from~\eqref{eq:CI_beta}
\begin{align*}
        {\beta_{k}(\delta)} &= C_w\sqrt{2\ln{\frac{2}{\delta}} + (n^2+nd)\ln\left(1 + \frac{HK\hat{\gamma}}{(n+d)\lambda_{min}}\right)}\nonumber\\
        & + \sqrt{\lambda_{max}} + \nu .
\end{align*}
Thus, we finally obtain that 
\begin{align*}
    &\mathcal{R}(K) \\
    = & O(H^{3/2}\sqrt{K})\\
    +& O\left(H\sqrt{K} (\sqrt{\lambda_{max}} + \nu) \sqrt{(n+d)\psi(\lambda_{min},n,d,H,K)} \right) \\
    +&O\left(H\sqrt{K}\left(\ln\frac{1}{\delta}+ n(n+d)\psi(\lambda_{min},n,d,H,K) \right)\right),
\end{align*}
in which
\begin{align*}
    \psi(\lambda_{min},n,d,H,K): =\ln\left(1+\frac{HK}{(n+d)\lambda_{min}}\right).
\end{align*}
\end{proof}

\subsection{Proofs of Lemmas for Theorem~\ref{thm:regret}}
\begin{proof}[Proof of Lemma~\ref{lem:regret_decomp}]
Let $\Gamma_{k,h}:= J_h^{\pi_k}(\Theta_*,x_{k,h}) - J_h^*(\widetilde{\Theta}_k,x_{k,h})$. 
\begin{align}
    R(K)& = \sum_{k=1}^K J_1^{\pi_k}(\Theta_*,x_{k,1}) - J_1^*(\Theta_*,x_{k,1})\nonumber\\
    & \lep{a} \sum_{k=1}^K J_1^{\pi_k}(\Theta_*,x_{k,1}) - J_1^*(\widetilde{\Theta}_k,x_{k,1})\nonumber\\
    & = \sum_{k=1}^K \Gamma_{k,1}\label{eq:sum_of_gamma},
\end{align}
where (a) holds by the optimistic algorithm (i.e.,~\eqref{eq:OFU}) under the event $\mathcal{E}_K(\delta)$.

To bound this, we first investigate $\Gamma_{k,h}$. Note that the action $u_{k,h}$ under $\pi_k$ is the same as that under an optimal policy when the true dynamics is $\widetilde{\Theta}$, and hence
\begin{align*}
    \Gamma_{k,h} = &\norm{x_{k,h}}_{Q_h} + \norm{u_{k,h}}_{R_h} + \ex{J_{h+1}^{\pi_k}(\Theta_*,x_{k,h+1}) \mid \mathcal{F}_{k,h}}\\
    -&\norm{x_{k,h}}_{Q_h} - \norm{u_{k,h}}_{R_h} - \sum_{h'=h+1}^{H}\ex{w_{h'}^\top P_{h'+1}(\widetilde{\Theta}_k) w_{h'}}\\
    -&\ex{ \norm{x_{k,h+1}}_{\tp_{k,h+1}} \mid \mathcal{F}_{k,h} }.
\end{align*}
Let $\widetilde{\psi}_{k,h+1}:= \sum_{h'=h+1}^{H}\ex{w_{h'}^\top P_{h'+1}(\widetilde{\Theta}_k) w_{h'}}$, we have
\begin{align*}
    \Gamma_{k,h} = &\ex{J_{h+1}^{\pi_k}(\Theta_*,x_{k,h+1}) \mid \mathcal{F}_{k,h}} - \widetilde{\psi}_{k,h+1} \\
    &-\ex{\norm{ \widetilde{\Theta}_k^\top z_{k,h} + w_{k,h}}_{\tp_{k,h+1}} \mid \mathcal{F}_{k,h}}\\
    =& \Delta_{k,h} + J_{h+1}^{\pi_k}(\Theta_*,x_{k,h+1}) - \widetilde{\psi}_{k,h+1}\\
    &-\ex{\norm{ \widetilde{\Theta}_k^\top z_{k,h} + w_{k,h}}_{\tp_{k,h+1}} \mid \mathcal{F}_{k,h}}
\end{align*}
where 
\begin{align*}
    \Delta_{k,h} := \mathbb{E}\left[J_{h+1}^{\pi_k}(\Theta_*,x_{k,h+1}) \mid \mathcal{F}_{k,h}\right] - J_{h+1}^{\pi_k}(\Theta_*,x_{k,h+1}).
\end{align*}
Now, by the assumptions on the noise (i.e., (b) in Assumption~\ref{ass:regularity}), we can write $\Gamma_{k,h}$ as follows. 
\begin{align*}
    &\Gamma_{k,h}\\
    \ep{a} & \Delta_{k,h} +  J_{h+1}^{\pi_k}(\Theta_*,x_{k,h+1}) - \widetilde{\psi}_{k,h+1} - \norm{\widetilde{\Theta}_k^\top z_{k,h}}_{\tp_{k,h+1}}\\
    &-\ex{\norm{w_{k,h}}_{\tp_{k,h+1}} \mid \mathcal{F}_{k,h}}\\
    =&\Delta_{k,h} +  J_{h+1}^{\pi_k}(\Theta_*,x_{k,h+1}) - \widetilde{\psi}_{k,h+1} - \norm{\widetilde{\Theta}_k^\top z_{k,h}}_{\tp_{k,h+1}}\\
    &-\ex{\norm{ x_{k,h+1} - \Theta_*^\top z_{k,h}   }_{\tp_{k,h+1}} \mid \mathcal{F}_{k,h}}\\
    \ep{b} & \Delta_{k,h} +  J_{h+1}^{\pi_k}(\Theta_*,x_{k,h+1}) - \widetilde{\psi}_{k,h+1} - \norm{\widetilde{\Theta}_k^\top z_{k,h}}_{\tp_{k,h+1}}\\
    &-\ex{\norm{ x_{k,h+1}  }_{\tp_{k,h+1}} \mid \mathcal{F}_{k,h}} + \norm{\Theta_*^\top z_{k,h}}_{\tp_{k,h+1}},\\
\end{align*}
where in (a) and (b), we have used the independence and mean zero of $w_{k,h}$.
In order to include the optimal cost term, we observe from~\eqref{eq:opt_cost} that 
\begin{align*}
    \widetilde{\psi}_{k,h+1} = J_h^*(\widetilde{M}_k,x_{k,h+1}) - \norm{x_{k,h+1}}_{\tp_{k,h+1}}.
\end{align*}

Based on this, we can further rewrite $\Gamma_{k,h}$ as
\begin{align}
     &\Gamma_{k,h}\nonumber\\
    = & \Delta_{k,h} +  J_{h+1}^{\pi_k}(\Theta_*,x_{k,h+1}) - J_{h+1}^*(\widetilde{\Theta}_k,x_{k,h+1}) \nonumber\\
    &+ \norm{x_{k,h+1}}_{\tp_{k,h+1}} -\ex{\norm{ x_{k,h+1}  }_{\tp_{k,h+1}} \mid \mathcal{F}_{k,h}}\label{eq:deltap}\\ 
    &+\norm{\Theta_*^\top z_{k,h}}_{\tp_{k,h+1}} - \norm{\widetilde{\Theta}_k^\top z_{k,h}}_{\tp_{k,h+1}}\label{eq:deltapp}\\
    =& \Delta_{k,h} + \Gamma_{k,h+1} + \Delta'_{k,h} + \Delta''_{k,h}\label{eq:final_decomp},
\end{align} 
in which~\eqref{eq:deltap} is denoted by $\Delta'_{k,h}$ and~\eqref{eq:deltapp} is denoted by $\Delta''_{k,h}$, respectively.

Finally, due to the fact that the cost for $H+1$ and beyond are zero, we can combine~\eqref{eq:sum_of_gamma} and~\eqref{eq:final_decomp} to obtain that 
\begin{align*}
    R(K) \le \sum_{k_1}^K\sum_{h=1}^{H-1} (\Delta_{k,h} + \Delta'_{k,h} + \Delta''_{k,h}),
\end{align*}
which completes the proof.
\end{proof}

\begin{proof}[Proof of Lemma~\ref{lem:two_Sum}]
We will bound both terms by using Azuma–Hoeffding inequality. Recall that $\mathcal{F}_{k,h}$ is  is all randomness \emph{before} time $(k,h)$, we have
\begin{align*}
    \ex{\Delta_{k,h} \mid \mathcal{F}_{k,h}} = 0 \text{ and } \ex{\Delta'_{k,h} \mid \mathcal{F}_{k,h}} = 0.
\end{align*}
Thus, all we need to show is that both of them are bounded.

\begin{align*}
    |\Delta'_{k,h}| &= \left|\norm{x_{k,h+1}}_{\widetilde{P}_{k,h+1}} - \mathbb{E}\left[\norm{x_{k,h+1}}_{\widetilde{P}_{k,h+1}} \mid \mathcal{F}_{k,h}\right]\right|\\
    &\le 2C,
\end{align*}
which follows from the boundness results in Lemmas~\ref{lem:fact_xz} and~\ref{lem:fact_P}.
To bound $|\Delta_{k,h}|$, we can bound it backwards by using the assumptions that $\norm{Q_h}_2\le C$ and $\norm{R_h}_2 \le C$. First notice that 
\begin{align*}
    |J_H^{\pi_k}(\Theta_*,x_{k,H})| &= \norm{x_{k,H}}_{Q_h} + \norm{u_{k,H}}_{R_h}\\
    &\le (1+\gamma^2)C,
\end{align*}
which again uses the boundness result in Lemma~\ref{lem:fact_xz}. 
Thus, for $h\in[H]$, we have 
\begin{align*}
    |J_h^{\pi_k}(\Theta_*,x_{k,H})| \le& \norm{x_{k,h}}_{Q_h} + \norm{u_{k,H}}_{R_h} \\
    &+ |\ex{J_{h+1}^{\pi_k}(\Theta_*,x_{k,h+1}) \mid \mathcal{F}_{k,h}}|\\
    \le& H(1+\gamma^2)C.
\end{align*}
Finally, a direct application of Azuma–Hoeffding inequality yields the result.
\end{proof}

\begin{proof}[Proof of Lemma~\ref{lem:thrid_Sum}]
    Note that
    \begin{align*}
        &\sum_{k=1}^K\sum_{h=1}^{H}\Delta''_{k,h} \le \sum_{k=1}^K\sum_{h=1}^{H}|\Delta''_{k,h}|\\
        =& \sum_{k=1}^K\sum_{h=1}^{H}\left| \norm{\tp_{k,h+1}^{1/2}\Theta_*^\top z_{k,h}}_2^2  - \norm{\tp_{k,h+1}^{1/2}\widetilde{\Theta}_k^\top z_{k,h}}_2^2 \right|\\
        \le & \left[ \sum_{k=1}^K\sum_{h=1}^{H}\left( \norm{\tp_{k,h+1}^{1/2}\Theta_*^\top z_{k,h}}_2 - \norm{\tp_{k,h+1}^{1/2}\widetilde{\Theta}_k^\top z_{k,h}}_2\right)^2 \right]^{1/2}\\
        &\cdot \left[ \sum_{k=1}^K\sum_{h=1}^{H}\left( \norm{\tp_{k,h+1}^{1/2}\Theta_*^\top z_{k,h}}_2 + \norm{\tp_{k,h+1}^{1/2}\widetilde{\Theta}_k^\top z_{k,h}}_2\right)^2 \right]^{1/2}.
    \end{align*}
    
    We will bound the two terms by using the following two claims, respectively.
    \begin{claim}
        Under Assumption~\ref{ass:regularity} and the event $\mathcal{E}_K(\delta)$, we have for some constant $D$
        \begin{align*}
            &\left[ \sum_{k=1}^K\sum_{h=1}^{H}\left( \norm{\tp_{k,h+1}^{1/2}\Theta_*^\top z_{k,h}}_2 + \norm{\tp_{k,h+1}^{1/2}\widetilde{\Theta}_k^\top z_{k,h}}_2\right)^2 \right]^{1/2} \\
            &\le 2D(1+\gamma) \sqrt{HK}.
        \end{align*}
    \end{claim}
    
    \begin{claim}
    \label{claim:C2}
        Under Assumption~\ref{ass:regularity} and the event $\mathcal{E}_K(\delta)$, we have for some constant $D$,
        \begin{align*}
            &\left[ \sum_{k=1}^K\sum_{h=1}^{H}\left( \norm{\tp_{k,h+1}^{1/2}\Theta_*^\top z_{k,h}}_2 - \norm{\tp_{k,h+1}^{1/2}\widetilde{\Theta}_k^\top z_{k,h}}_2\right)^2 \right]^{1/2} \\
            &\le 2HD(1+\gamma)\beta_k(\delta)\left( \ln\frac{\det(G_k+\lambda_{min} I)}{\det( \lambda_{min}I )}\right)^{1/2} .
        \end{align*}
    \end{claim}
    
\end{proof}

\subsection{Proofs for Claims}
\begin{proof}[Proof of Claim~\ref{claim:C2}]
     Under Assumption~\ref{ass:regularity} and the event $\mathcal{E}_K(\delta)$, we have
     \begin{align*}
         &\left( \norm{\tp_{k,h+1}^{1/2}\Theta_*^\top z_{k,h}}_2 - \norm{\tp_{k,h+1}^{1/2}\widetilde{\Theta}_k^\top z_{k,h}}_2\right)^2\\
         \le & \norm{\tp_{k,h+1}^{1/2}(\widetilde{\Theta}_k-\Theta_* )^\top z_{k,h} }_2^2 \\
         \lep{a} & D^2\norm{(\widetilde{\Theta}_k-\Theta_* )^\top z_{k,h}}_2^2\\
         \le & D^2\norm{(\widetilde{\Theta}_k-\Theta_* )^\top \hat{V}_k^{1/2}  }_2^2 \norm{\hat{V}_k^{-1/2} z_{k,h} }_2^2\\
         \le & 2D^2\beta_k^2(\delta)\norm{\hat{V}_k^{-1/2} z_{k,h} }_2^2.
     \end{align*}
     
Combining the result above with the boundeness of $\tp_{k,h+1}$, $\Theta_*$, $\widetilde{\Theta}_k$ and $z_{k,h}$, yields
\begin{align*}
    &\norm{\tp_{k,h+1}^{1/2}(\widetilde{\Theta}_k-\Theta_* )^\top z_{k,h} }_2^2\\
    \lep{a} &2D^2(1+\gamma)^2 \beta_{k}^2(\delta) \min\left\{1,\norm{\hat{V}_k^{-1/2} z_{k,h} }_2^2 \right\}\\
    \lep{b}&2D^2(1+\gamma)^2 \beta_{k}^2(\delta) \min\left\{1,\norm{ z_{k,h} }_{(G_k+\lambda_{min})^{-1}}^2 \right\}\\
    \lep{c}&4D^2(1+\gamma)^2 \beta_{k}^2(\delta) \ln\left( 1+ \norm{ z_{k,h} }_{(G_k+\lambda_{min})^{-1}}^2 \right).
\end{align*}

Thus, we have 
\begin{align*}
    &\sum_{k=1}^K\sum_{h=1}^{H}\left( \norm{\tp_{k,h+1}^{1/2}\Theta_*^\top z_{k,h}}_2 - \norm{\tp_{k,h+1}^{1/2}\widetilde{\Theta}_k^\top z_{k,h}}_2\right)^2\\
    \le & \sum_{k=1}^K\sum_{h=1}^{H}8D^2(1+\gamma)^2 \beta_{k}^2(\delta) \ln\left( 1+ \norm{ z_{k,h} }_{(G_k+\lambda_{min})^{-1}}^2 \right)\\
    \lep{a}& 4(H)D^2(1+\gamma)^2 \beta_{k}^2(\delta) \ln\frac{\det(G_k+\lambda_{min} I)}{\det( \lambda_{min}I )}.
\end{align*}
Taking the square root complemtes the proof.

\end{proof}

\subsection{Lemmas for Private Control}
% We will inject Gaussian noise to protect $z_t z_t^T$ and $z_t x_{t+1}^T$ by adding $N_t \in \mathbb{R}^{n+d \times n+d}$ and $M_t \in \mathbb{R}^{n+d \times n}$, respectively. More specifically, we will send $z_t z_t^T + N_t$ and $z_t x_{t+1}^T + M_t$ to the server at each step $t$. We require that $N_t(i,j) \stackrel{i.i.d}{\sim} \mathcal{N}(0,\sigma_1^2)$ for all $i \le j$ and $N_t(j,i) = N_t(i,j)$, $M_t(i,j)\stackrel{i.i.d}{\sim} \mathcal{N}(0,\sigma_2^2)$ for all $i, j$, where $\sigma_1$ and $\sigma_2$ are constants determined by the requirement of LDP privacy in Task 1.

% Thus, we have $H_t = \sum N_t + cI$ and $K_t =\sum M_t$, where we need to add an additional $cI$, $c>0$ to ensure that $H_t$ is PSD.

\begin{lemma}[Slepian’s inequality; Lemma 5.33 in~\cite{vershynin2010introduction}]
\label{lem:Slepian}
    Consider two Gaussian processes $(X_t)_{t\in T}$ and $(Y_t)_{t\in T}$ whose increments satisfy the inequality $\ex{|X_s -X_t|^2} \le \ex{|Y_s - Y_t|^2}$ for all $s, t\in T$, then, $\ex{\sup_{t\in T} X_t}  \le \ex{\sup_{t\in T}Y_t}$.
\end{lemma}

\begin{lemma}[Concentration in the Gauss space]
\label{lem:cgauss}
    Let $f$ be a real valued $1$-Lipschitz function on $\mathbb{R}^n$. Let $X$ be a Gaussian random vector in $\mathbb{R}^n$ whose entries $X_i$ is $i.i.d$ $\mathcal{N}(0,\sigma^2)$. Then, for every $t\ge 0$,
    \begin{align*}
        \mathbb{P}\left\{f(X) - \ex{f(X)} \ge t \right\} \le \exp\left(-\frac{t^2}{2\sigma^2}\right)
    \end{align*}
\end{lemma}
\begin{proof}
    This result directly follows from Proposition 2.18 in~\cite{ledoux2001concentration} by considering $\gamma$ as the Gaussian measure on $\mathbb{R}^n$ with density of a multivariate normal distribution, i.e., $\mathcal{N}{(0,\sigma^2 I)}$ and hence $c$ in Proposition 2.18 of~\cite{ledoux2001concentration} is equal to $\frac{1}{\sigma^2}$. 
\end{proof}

\begin{lemma}[Operator norm of Gaussian random matrices]
\label{lem:norm_gaussian}
    Let $A$ be an $m \times n$ random matrix whose entries $A_{ij}$ are $i.i.d$ Gaussian random variables $\mathcal{N}(0,\sigma^2)$. Then, for any $t>0$, we have 
    \begin{align*}
        \mathbb{P}\{\norm{A} \ge \sigma(\sqrt{n} +\sqrt{m}) +t\} \le \exp\left(-\frac{t^2}{2\sigma^2}\right).
    \end{align*}
\end{lemma}
\begin{proof}
    We will first show that 
    \begin{align*}
        \ex{\norm{A}} \le \sigma(\sqrt{m} + \sqrt{n})
    \end{align*}
    by using Lemma~\ref{lem:Slepian}. To this end, note that the operator norm of $A$ can be computed as follows.
    \begin{align*}
        \norm{A} = \max_{u \in S^{n-1}, v\in S^{m-1}}\inner{Au}{v}.
    \end{align*}
    where $S^{n-1}$ and $s^{m-1}$ are unit spheres. Thus, $\norm{A}$ can be regarded as the supremum of the Gaussian process $X_{u,v}:=\inner{Au}{v}$ indexed by the pair of vectors $(u,v)\in S^{n-1} \times S^{m-1}$. Let us define $Y_{u,v}:=\inner{g}{u} + \inner{h}{v}$ where $g\in \mathbb{R}^n$ and $h \in \mathbb{R}^m$ are independent Gaussian random vectors whose entries are $i.i.d$ Gaussian random variables $\mathcal{N}(0,\sigma^2)$. Now, we compare the increments of these two Gaussian processes for every $(u,v),(u',v') \in S^{n-1} \times S^{m-1}$.
    \begin{align*}
        &\ex{|X_{u,v} -X_{u',v'}|^2}\\ &= \sigma^2\sum_{i=1}^n\sum_{j=1}^m |u_iv_j -u'_iv'_j|^2\\
        &=\sigma^2\norm{uv^T - u'v'^T}_{F}^2\\
        &=\sigma^2\norm{(u-u')v^T + u'(v-v')^T}_{F}^2\\
        &=\sigma^2\left(\norm{u-u'}_2^2 + \norm{v-v'}_2^2\right)\\
        & \quad+  2\sigma^2\text{trace}\left(v(u-u')^Tu'(v-v')^T\right)\\
        &=\sigma^2\left(\norm{u-u'}_2^2 + \norm{v-v'}_2^2 + 2(u^Tu' -1)(1-v^Tv') \right)\\
        &\le \sigma^2\left(\norm{u-u'}_2^2 + \norm{v-v'}_2^2\right)\\
        &= \ex{|Y_{u,v} -Y_{u',v'}|^2}.
    \end{align*}
    Therefore, Lemma~\ref{lem:Slepian} applies here, and hence
    \begin{align*}
        \ex{\norm{A}}& = \ex{\max_{(u,v)}{X_{u,v}}} \le \ex{\max_{(u,v)}{Y_{u,v}}}\\
        &= \ex{\norm{g}_2} + \ex{\norm{h}_2} \le \sigma(\sqrt{m} + \sqrt{n}).
    \end{align*}
    Finally, note that $\norm{A}$ is a $1$-Lipschitz function of $A$ when considered as a vector in $\mathbb{R}^{mn}$. Then, consider the function $f$ in Lemma~\ref{lem:cgauss} as the operator norm, we directly obtain the result.
 \end{proof}   
 
\begin{lemma}[Operator norm of symmetric Gaussian random matrices]
\label{lem:norm_sym_gaussian}
    Let $A$ be an $n \times n$ random symmetric matrix whose entries $A_{ij}$ on and above the diagonal are $i.i.d$ Gaussian random variables $\mathcal{N}(0,\sigma^2)$. Then, for any $t>0$, we have \begin{align*}
        \norm{A} \le 4\sigma\sqrt{n} + 2t,
    \end{align*}
    with probability at least $1-2\exp(-\frac{t^2}{2\sigma^2})$.
\end{lemma} 
 \begin{proof}
     Decompose the matrix $A$ into the upper triangular matrix $A^+$ and the lower triangular matrix $A^-$ such that $A = A^+ + A^-$. Note that without loss of generality, the entries on the diagonal are in $A^+$. Then, apply Lemma~\ref{lem:norm_gaussian} to both $A^+$ and $A^-$, and by a union bound, we have that the following inequalities hold simultaneously 
     \begin{align*}
         \norm{A^+} \le 2\sigma\sqrt{n} + t \quad\text{and}\quad \norm{A^-} \le 2\sigma\sqrt{n} + t
     \end{align*}
    with probability at least $1-2\exp(-\frac{t^2}{2\sigma^2})$ for any $t > 0$. Finally, by triangle inequality $\norm{A} \le \norm{A^+} + \norm{A^-}$, we prove the result.
 \end{proof}
 \begin{lemma}[Concentration of chi-square; Corollary to Lemma 1 of~\cite{laurent2000adaptive}]
 \label{lem:chi-square}
    Let $U$ be a $\chi^2$ statistic with $D$ degrees of freedom. Then, for any positive $x$,
    \begin{align*}
        \mathbb{P}\left\{ U \ge D + 2\sqrt{Dx} + 2x\right\} \le \exp(-x).
    \end{align*}
 \end{lemma}
